# Supplementary material for: From Dataset Recycling to Multi-Property Extraction and Beyond
Source: arXiv:2011.03228 source file (2020-11-06)
Supplement: Supplementary file 1 [file the-appendix.tex]

\documentclass[11pt,a4paper]{article}
\usepackage[hyperref]{emnlp2020}
\usepackage{times}
\usepackage{latexsym}

\usepackage{microtype}
\usepackage{comment}
\usepackage{placeins}
\usepackage{float}
\aclfinalcopy %

\input{extras}
\input{preamble}
\usepackage{tabularx}

\usepackage{multicol}

\begin{document}

\input{appendix}

\end{document}
